# Supplementary material for: Proof-of-Stake Mining Games with Perfect Randomness
Source: arXiv:2107.04069 source file (2021-12-14)
Supplement: Supplementary file 1 [file nash-others.tex]

\documentclass[../main.tex]{subfiles}

\begin{document}

The next example highlights the intuition behind our proof.
\begin{example}
Consider state $B_{1, 1} = ((\{0, 2\}, \{2 \to 0\}), \{1\}, \{1\})$ and its $1$-Capitulation is the state $B_0$. We will give a proof sketch for showing $V(B) \leq 1$. The idea is to observe that $B_{1, 1}$ is similar to $B_0$ when we restrict our attention to only blocks that can reach height $\geq 2$. Consider the coupling between the mining games;
\begin{itemize}
\item The first game starts at state $X_0 = B_{1, 1}$ and Miner 1 follows an arbitrary optimal positive recurrent strategy $\pi$.
\item The second mining game starts at state $X_0' = B_0$ and Miner 1 follows strategy $\pi'$ (that will depend on $\pi$).
\end{itemize}
Miner 1 creates block $n \geq 3$ with probability $\alpha$. Additionally, Miner $k$ creates block $n \geq 3$ in the first game if and only if Miner $k$ creates block $n$ in the second game.

Define $\pi'$ to capitulate to state $B_0$ whenever $\pi$ capitulates to state $B_0$. Let $\tau$ be the first time step $\pi$ capitulates to state $B_0$. We will define strategy $\pi'$ such that we can ensure  the longest path in the second game at heights $\geq 2$ is {\em always} identical to the longest path in the first game at heights $\geq 1$. For that, $\pi'$ copies all actions of $\pi$ except when $\pi$ plays $\publishpath(Q, v)$ and $1 \in Q$ or $h(v) \leq 1$.

For example, assume Miner 1 creates block 3 and 4 and Miner 2 creates block 5. Then $\pi$ publishes $4 \to 3 \to 1 \to 0$ forking blocks 2 and 5. $\pi'$ cannot take the same action since block 1 is not one of Miner 1 unpublished blocks. Instead, $\pi'$ publishes $4 \to 3 \to 0$ forking block 5. At time $\tau$, the longest path of the first game at height $\geq 2$ is identical to the longest path of the second game at height $\geq 1$. Thus the only advantage Miner 1 has in the first game compared with the second game is the possibility that block 1 is a block in the longest path. Let $p$ be the probability block 1 is part of the longest path in the first game. Then, the value function of the first game is
$$V(B_{1, 1}) = \e{r_{\lambda^*}(X_0, X_\tau) | X_0 = B_{1, 1}}= \e{r_{\lambda^*}(X_0', X_\tau') | X_0' = B_0} + p$$
where $\lambda^* = \max_\pi \rev(\pi)$. From Bellman's Principle of Optimality (Lemma~\ref{lemma:bellman}),
$$V(B_{1, 1}) =  \e{r_{\lambda^*}(X_0', X_\tau') | X_0' = B_0} + p \leq V(B_0) + p \leq 1$$
where the last inequality observes $V(B_0) = 0$ and $p \leq 1$.
\end{example}
\begin{observation}\label{obs:path-independence} $\rew(X_t, X_{t+1}) + \rew(X_{t+1}, X_{t+2}) = \rew(X_t, X_{t+1})$
\end{observation}
\begin{proof}
Follows directly from the definition of $r_\lambda$:
\begin{align*}
\rew(X_t, X_{t+1}) &:= (1-\lambda)\left(|A(\chain(X_{t+1})) \cap T_1| - |A(\chain(X_t)) \cap T_1|\right)\\
&\qquad - \lambda \left(|A(\chain(X_{t+1})) \cap T_2| - |A(\chain(X_t)) \cap T_2|\right).
\end{align*}
\end{proof}
This coupling causes the longest path in $(X_t)_{t\geq 0}$ (at heights $c + 1, c+2, \ldots$) to be {\em equal} to the longest path in $(X_t')_{t \geq 0}$ (at heights $1, 2, \ldots$). Let $D$ be the blocks that could not reach height $\geq c + 1$ from state $B$ -- that is, $B' = B[V(B) \setminus D]$.
\begin{claim}
For all $t \geq 0$, $\Succ(H_c(X_t)) = A(\chain(X_t'))\setminus \{0\}$ and $\unpublished(X_t) \setminus D \subseteq \unpublished(X_t')$.
\end{claim}
\begin{proof}
The proof is by induction on $t$. The base case $t = 0$ is clear from the definition of $B'$. For the inductive step, it suffices to consider the time step $t \geq 1$ where $\pi$ plays $\publishpath(Q, v)$. Let's first check that $Q'$ are blocks that $\pi'$ can publish at time $t$. Recall $D$ contain all the blocks in state $B$ that cannot reach height $\geq c + 1$ and $Q'$ contain only blocks that reach height $\geq c + 1$. Thus, $Q' \cap D = \emptyset$. Because $Q \subseteq \unpublished(X_{t-1})$ (since $\publishpath(Q, v)$ is a valid action), we conclude
$$Q' \subseteq \unpublished(X_{t-1}) \setminus D \subseteq \unpublished(X_{t-1}')$$
where the last $\subseteq$ is the inductive hypothesis. This proves $\pi'$ can publish $Q'$ at time $t$. If $\pi$ publishes $Q$ and $\pi'$ publishes $Q'$, then from the inductive hypothesis,
$$\unpublished(X_t) \setminus D = \unpublished(X_{t-1}) \setminus D \setminus Q \subseteq \unpublished(X_{t-1}') \setminus Q' = \unpublished(X_t')$$
since $Q' \subseteq Q$. To show $\Succ(H_c(X_t)) = A(\chain(X_t'))$, we consider separately the case where $h(v) > c$ and the case where $h(v) \leq c$.

\vspace{1mm}\noindent\textbf{Case 1:} Assume $h(v) > c$. Note $v$ is in the longest path (because $\pi$ is LCM). Thus $v \in \Succ(H_c(X_{t-1})) = A(\chain(X_{t-1}')) \setminus \{0\}$ where the equality is the inductive hypothesis. Thus $\publishpath(Q', v)$ is a valid action for $\pi'$. Additionally, $Q = Q'$ since all blocks in $Q$ have height $\geq c +1$ once $\pi$ plays $\publishpath(Q, v)$. From the inductive hypothesis, the successors $\Succ(v)$ of $v$ in both games are identical. Since $\pi$ is timeserving,
$$|Q| \geq |\Succ(v)| + 1.$$
Thus $\publishpath(Q', v) = \publishpath(Q, v)$ is timeserving for $\pi'$ and forks the longest chain $\chain(X_{t-1}')$. After both $\pi$ and $\pi'$ takes action $\publishpath(Q, v)$, 
$$\Succ(H_c(X_t)) = A(\chain(X_t')) \setminus \{0\}.$$
This proves the inductive step for the case $h(v) > c$.

\vspace{1mm}\noindent\textbf{Case 2:} Assume $h(v) \leq c$. After taking action $\publishpath(Q, v)$, $\pi$ forks all blocks in $\Succ(H_c(X_{t-1}))$ (because $\pi$ is timeserving). Thus
$$\Succ(H_c(X_t)) = Q'.$$
Because $\pi$ forks the longest chain,
$$|Q'| = |\Succ(H_c(X_t))| \geq |\Succ(H_c(X_{t-1}))| + 1 = h(\chain(X_{t-1}')) + 1$$
where the inequality is from the fact $\pi$ forks the longest chain $\chain(X_{t-1})$ and last equality is from the inductive hypothesis. Thus $\publishpath(Q', 0)$ is a valid action for $\pi'$ that forks the longest chain $\chain(X_{t-1}')$. After taking such action,
$$A(\chain(X_t')) \setminus \{0\} = Q'.$$
This proves the inductive step for the case $h(v) \leq c$.
\end{proof}

\begin{proposition}\label{prop:b_2_0}
For $\alpha < \frac{1}{2}(3-\sqrt{5})$, $V(B_{2, 0}) = \big(2+\frac{\alpha}{1-2\alpha}\big)(1-\lambda^*)$.
\end{proposition}
\begin{proof}\def\currentprefix{prop:b_2_0}
We will show the $\sm$ (Definition~\ref{def:selfish-mining}) is an optimal strategy for a mining game starting from state $B_{2, 0}$. Define the mining game starting at state $X_0 = B_{2, 0}$ where Miner 1 follows the $\sm$ strategy. At time $t \geq 1$, Miner 1 creates block $t + 2$ with probability $\alpha$; otherwise, Miner 2 creates block $t + 2$. Let $\tau \geq 1$ be the first time step where Miner 1 capitulates to state $B_0$. Recall, for the selfish mining strategy,
$$\tau = \min\{t \geq 0 : |T_2(X_t)| = |T_1(X_t)| - 1\}$$
because Miner 1 waits until the first time step where its advantage reduces to a single block to subsequently fork all of Miner 2 blocks. Thus $X_\tau^\half$ is the state Miner 1 is about to fork $T_2(X_t)$ and $X_\tau$ is the state after Miner 1 forks $T_2(X_t)$. That is,
$$X_\tau^\half = (\gpath(\{0\} \cup T_2(X_\tau)), T_1(X_\tau), T_1(X_\tau)).$$
$$X_\tau = (\gpath(\{0\} \cup T_1(X_\tau)), \emptyset, T_1(X_\tau)).$$
Because Miner 1 receives $T_1(X_\tau)$ blocks and Miner 2 receives no blocks,
$$r_{\lambda^*}(X_0, X_\tau) = T_1(X_\tau)(1-\lambda^*).$$
\begin{claim}\label{claim:b_2_0}
$V(B_{2, 0}) \geq V_\sm^{\lambda^*}(B_{2, 0}) = \left(2 + \frac{\alpha}{1-2\alpha}\right)(1-\lambda^*)$.
\end{claim}
\begin{proof}
From Lemma~\ref{lemma:bellman},
\begin{equation}
V(B_{2, 0}) \geq V_\sm^{\lambda^*}(B_{2,0}) = \e{r_{\lambda^*}(X_0, X_\tau)} = \e{T_1(X_\tau)}(1-\lambda^*) = \left(2+\frac{\alpha}{1-2\alpha}\right)(1-\lambda^*).
\end{equation}
where last Equality is from Lemma~\ref{lemma:selfish-mining-reward}.
\end{proof}
Let $\pi^*$ be an optimal, trimmed, positive recurrent strategy. Define a mining game starting at state $X_0' = B_{2, 0}$ where Miner 1 uses strategy $\pi^*$. We will define a coupling between $(X_t')_{t \geq 0}$ and $(X_t)_{t \geq 0}$. At time $t \geq 1$, Miner $k$ creates block $t + 2$ in game $(X_t)_{t \geq 0}$ if and only if Miner $k$ creates block $t + 2$ in game $(X_t')_{t \geq 0}$. Let $\tau' \geq 1$ be the first time step where Miner 1 capitulates to state $B_0$ (in game $(X_t')_{t \geq 0}$). Assume $\sm$ is not an optimal strategy for a game starting at state $B_{2, 0}$; otherwise, $V(B_{2, 0}) = V_\sm^{\lambda^*}(B_{2, 0})$ and we are done.
\begin{claim}\locallabel{claim:1}
For all $1 \leq t \leq \tau$, Miner 2 creates more blocks than Miner 1 from time $t$ to $\tau$ (including time $t$ and $\tau$).
\end{claim}
\begin{proof}
Observe $|T_1(X_0)| = |T_2(X_0)| - 2$ and $|T_1(X_\tau) = |T_2(X_\tau)| - 1$. If Miner 1 creates at least the same number of blocks as Miner 2 from time $t$ to $\tau$, there is a time $1 \leq t' < \tau$ such that $|T_1(X_{t'})| = |T_2(X_{t'})| - 1$, a contradiction to $\tau$ being the first time step $\geq 1$ where $|T_1(X_\tau)| = |T_2(X_\tau)| - 1$.
\end{proof}
\begin{claim}\locallabel{claim:2}
At time $\tau$, $\publishpath(T_1(X_\tau), 0)$ is the unique valid action for Miner 1 that can fork the longest chain $\chain(X_\tau^\half)$.
\end{claim}
\begin{proof}
It is clear $\publishpath(T_1(X_\tau), 0)$ is a valid action for Miner 1 that can fork the longest chain $\chain(X_\tau^\half)$. It is also clear that if $\publishpath(Q, 0)$ is another valid action then $Q = T_1(X_\tau)$ if Miner 1 hopes to fork the longest chain. Suppose for contradiction, there is an action $\publishpath(Q, v)$ with $v \geq 1$ that can fork the longest chain. Then
$$|\unpublished(X_\tau^\half) \cap (v, \infty)| \geq |\Succ(v)| + 1.$$
Observe $v \leq \tau - 1$ because Miner 2 creates block $\tau$. Because $\unpublished(X_\tau^\half) = T_1(X_\tau)$ and $A(\chain(X_\tau^\half))\setminus \{0\} = T_2(X_\tau)$, the fact Miner 1 forks the longest chain by taking $\publishpath(Q, v)$ implies
$$|T_1(X_\tau) \cap (v, \infty)| \geq |T_2(X_\tau) \cap (v, \infty)| + 1 \Longrightarrow\Longleftarrow.$$
The last line contradicts the fact Miner 2 creates more blocks than Miner 1 from time $v+1 \leq \tau$ to $\tau$ (Claim~\localref{claim:1}). This proves there is no alternative action to $\publishpath(T_1(X_\tau), 0)$ that can fork the longest chain at time $\tau$.
\end{proof}
Claim~\localref{claim:2} gives intuition why publishing $T_1(X_\tau)$ at time $\tau$ is optimal. Suppose Miner 1 does not publish $T_1(X_\tau)$ at time $\tau$ and Miner 2 creates block $\tau+1$ (with probability $1-\alpha$). Then Claim~\localref{claim:2} implies Miner 1 does not have enough blocks to publish $T_1(X_\tau)$. From the Tie Breaking Lemma~\ref{lemma:tie-breaking}, the probability that Miner 1 will have another opportunity to publish $T_1(X_\tau)$ is at most $\alpha/(1-\alpha)$. For small values of $\alpha$, the risk of losing $T_1(X_\tau)$ is too high and, as we will see, Miner 1 would prefer to publish $T_1(X_\tau)$ at time $\tau$.

Consider the following events partitioning the probability space:
\begin{itemize}
\item $E_1$: $\tau' \leq \tau$.
\item $E_2$: $\tau' > \tau$ and Miner 1 (in game $(X_t')_{t \geq 0}$) publishes blocks up to time $\tau$.
\item $E_3$: $\tau' > \tau$ and Miner 1 (in game $(X_t')_{t \geq 0}$) does not publishes any blocks up to time $\tau$.
\end{itemize}
\begin{claim}\locallabel{claim:3} $\e{r_{\lambda^*}(X_0', X_{\tau'}') | E_1} \leq \e{r_{\lambda^*}(X_0, X_\tau) | E_1}.$
\end{claim}
\begin{proof}
Note $r_{\lambda^*}(X_0', X_{\tau'}')$ is maximum when Miner 1 publishes all blocks they create up to time $\tau'$ and Miner 2 publishes no blocks they create up to time $\tau'$. Thus
$$r_{\lambda^*}(X_0', X_{\tau'}') \leq |T_1(X_{\tau'}')|(1-\lambda^*) \leq |T_1(X_\tau)|(1-\lambda^*) = r_{\lambda^*}(X_0, X_\tau).$$
\end{proof}
\begin{claim}\locallabel{claim:4} $\e{r_{\lambda^*}(X_0', X_{\tau '}') | E_2} \leq \e{r_{\lambda^*}(X_0, X_\tau) | E_2}$.
\end{claim}
\begin{proof}
Event $E_2$ implies $\tau' > \tau$. Thus
$$\e{r_{\lambda^*}(X_0', X_{\tau'}')|E_2} = \e{r_{\lambda^*}(X_0', X_{\tau}') + r_{\lambda^*}(X_\tau', X_{\tau'}') | E_2} = \e{r_{\lambda^*}(X_0', X_\tau') + V(X_\tau') | E_2}$$
where the first equality is Observation~\ref{obs:path-independence}. Event $E_2$ implies Miner 1 has at least one block in the longest path at time step $\tau$. Thus the height of the longest chain at time $\tau$ is
$$h(\chain(X_\tau')) \geq |T_2(X_\tau)| + 1 = |T_1(X_\tau)| = h(\chain(X_\tau)).$$
Next, we consider separately the case where $h(\chain(X_\tau')) = |T_1(X_\tau)|$ and the case where $h(\chain(X_\tau')) \geq |T_1(X_\tau)| + 1$.

\vspace{1mm}\noindent\textbf{Case 1.} Consider the case where $h(\chain(X_\tau')) = |T_1(X_\tau)|$. Recall $\publishpath(T_1(X_\tau), 0)$ is the unique action for Miner 1 that could fork the longest chain at time $\tau$ (Claim~\localref{claim:2}. Therefore, Miner 1 has no blocks that can reach height $> h(\chain(X_\tau'))$ and the $h(\chain(X_\tau'))$-Capitulation of state $X_\tau'$ is state $B_0$. From Lemma~\ref{lemma:truncation},
\begin{align*}
r_{\lambda^*}(X_0', X_\tau') + V(X_\tau') &\leq \sum_{i = 1}^{|T_1(X_\tau)|} Pr[H_i(X_{\tau'}') \in T_1] - |T_1(X_\tau)|\lambda^*\\
&\leq |T_1(X_\tau)|(1-\lambda^*) = r_{\lambda^*}(X_0, X_\tau).
\end{align*}

\vspace{1mm}\noindent\textbf{Case 2.} Consider the case $h(\chain(X_\tau')) \geq |T_1(X_\tau)| + 1$. Recall Miner 2 publishes only $|T_2(X_\tau)|$ blocks up to time $\tau$ and $|T_1(X_\tau)| = |T_2(X_\tau)| + 1$. Therefore, Miner 1 published at least two blocks up to time $\leq \tau$. We claim that Miner 1 needs two blocks to fork the longest chain $\chain(X_\tau')$. For that, it suffices to show that for any $v \in A(\chain(X_\tau'))$, $|\Succ(v)| \geq |\unpublished(X_\tau') \cap (v, \infty)| + 1$. For the case $v \geq 2$, recall Miner 2 creates more blocks than Miner 1 from time $v + 1$ to time $\tau$ (Claim~\localref{claim:1}). Thus
$$\Succ(v) \geq |T_2(X_\tau) \cap (v, \tau]| \geq |T_1(X_\tau) \cap (v, \tau]| +1 \geq |\unpublished(X_\tau') \cap (v, \infty)| + 1$$
For the case where $v \in \{0, 1\}$, observe Miner 1 created at least one block in $\Succ(v)$ (because Miner 1 has at least two blocks in the longest path). Thus
$$|\Succ(v)| \geq |T_2(X_\tau) \cap (v, \tau]| + 1 \geq |T_1(X_\tau) \cap (v, \tau]| + 1 \geq |\unpublished(X_\tau') \cap  (v, \infty)| + 1.$$
Both cases proves Miner 1 needs at least two blocks to fork the longest chain $\chain(X_\tau')$ and the $h(\chain(X_\tau'))$-Capitulation of $X_\tau'$ is the state $B_0$. From Lemma~\ref{lemma:truncation},
$$r_{\lambda^*}(X_0', X_\tau') + V(X_\tau') \leq \sum_{i = 1}^{h(\chain(X_\tau'))} \pr{H_i(X_{\tau'}') \in T_1} - h(\chain(X_\tau'))\lambda^*.$$
Let $M_k = A(\chain(X_\tau')) \cap T_k$ denote the blocks in the longest chain created by Miner $k$. For each $v \in M_2$, the probability Miner 1 forks block $v$ is at most the probability that Miner 1 forks the longest chain $\chain(X_\tau')$. From the Tie Breaking Lemma~\ref{lemma:tie-breaking}, the probability of Miner 1 forking $\chain(X_\tau')$ is at most $(\alpha/(1-\alpha))^2$ (because Miner 1 needs two blocks to fork $\chain(X_\tau')$). Thus
\begin{align*}
\sum_{i = 1}^{h(\chain(X_\tau'))} Pr[H_i(X_t') \in T_1] - \ell\lambda^* &\leq |M_1| + |M_2|\left(\frac{\alpha}{1-\alpha}\right)^2 - \ell \lambda^*\\
&= |M_1|(1-\lambda^*) + |M_2|\left(\left(\frac{\alpha}{1-\alpha}\right)^2-\lambda^*\right).
\end{align*}
Recall $\lambda^* \geq \alpha$ (because the revenue of $\frontier$ is $\alpha$ and $\lambda^* = \max_\pi \rev(\pi)$). For $\alpha < \frac{3-\sqrt{5}}{2}$,
$$\left(\frac{\alpha}{1-\alpha}\right)^2 - \alpha \leq 0.$$
Therefore,
$$r_{\lambda^*}(X_0', X_\tau') + V(X_\tau') \leq |M_1|(1-\lambda^*) \leq |T_1(X_\tau)|(1-\lambda^*) = r_{\lambda^*}(X_0, X_\tau).$$
Case 1 and 2 proves $r_{\lambda^*}(X_0', X_\tau') + V(X_\tau') \leq r_{\lambda^*}(X_0, X_\tau)$. This proves $\e{r_{\lambda^*}(X_0', X_\tau') | E_2} \leq \e{r_{\lambda^*}(X_0, X_\tau) | E_2}$.
\end{proof}
\begin{claim}\locallabel{claim:5}
If $\sm$ is not an optimal strategy for a mining game starting at state $B_{2,0}$, then $\e{r_{\lambda^*}(X_0', X_{\tau'}') | E_3} \leq \e{r_{\lambda^*}(X_0, X_\tau) | E_3}$.
\end{claim}
\begin{proof}
Event $E_3$ implies $\tau' > \tau$. Thus
$$\e{r_{\lambda^*}(X_0', X_{\tau'}') | E_3} = \e{r_{\lambda^*}(X_0', X_\tau') + r_{\lambda^*}(X_\tau', X_{\tau'}') | E_3} = \e{r_{\lambda^*}(X_0', X_\tau') + V(X_\tau') | E_3}$$
where the first equality is Observation~\ref{obs:path-independence}. Event $E_3$ implies Miner 1 does not publish blocks up to time $\tau$. Thus
$$X_\tau' = X_\tau = (\gpath(\{0\} \cup T_2(X_\tau)), T_1(X_\tau), T_1(X_\tau)).$$
We will divide the proof into two cases depending on whom creates block $\tau + 3$ at time step $\tau + 1$. Let $Z_1$ be the state immediately after $X_\tau'$ when Miner 1 creates block $\tau + 3$. Let $Z_2$ be the state immediately after $X_\tau'$ when Miner 2 publishes $\tau + 3 \to \chain(X_\tau')$. That is,
$$Z_1 = (\gpath(\{0\} \cup T_2(X_\tau)), T_1(X_\tau) \cup \{\tau + 3\}, T_1(X_\tau) \cup \{\tau + 3\}).$$
$$Z_2 = (\gpath(\{0\} \cup T_2(X_\tau) \cup \{\tau+3\}),  T_1(X_\tau), T_1(X_\tau)).$$
Recall the only action for Miner 1 that forks the longest chain at time $\tau$ is $\publishpath(T_1(X_\tau), 0)$ (Claim~\localref{claim:2}). Thus if Miner 2 publishes $\tau + 3 \to \chain(X_\tau')$, Miner 1 has no actions to fork the new longest chain $\tau + 3$. Therefore, the $|T_1(X_{\tau})|$-Capitulation of state $Z_2$ is the state $B_0$. From Lemma~\ref{lemma:truncation},
$$r_{\lambda^*}(X_0', Z_2) + V(Z_2) \leq \sum_{i = 1}^{|T_1(X_{\tau})|} \pr{H_i(X_{\tau'}') \in T_1} - |T_1(X_{\tau})|\lambda^*. $$
Clearly $\pr{H_i(X_t') \in T_1} \leq \pr{H_{i+1}(X_t') \in T_1}$, for $i < |T_1(X_{\tau})|$, since Miner 1 must fork the block at height $i+1$ to fork a block at height $i$. From Lemma~\ref{lemma:tie-breaking}, the probability Miner 1 forks the block at height $|T_1(X_{\tau})|$ is at most $p = \frac{\alpha}{1-\alpha}$. Thus
\begin{equation}\locallabel{eq:z_2}
r_{\lambda^*}(X_0', Z_2) + V(Z_2) \leq |T_1(X_{\tau})|(p-\lambda^*).
\end{equation}
Next, we upper bound $r_{\lambda^*}(X_0', Z_1) + V(Z_1)$. Let $b_1 = \max\ T_1(X_\tau)$ and $b_2 = \tau + 3$. From Claim~\localref{claim:2}, $b_1$ and $b_2$ are the only blocks Miner 1 can publish at height $|T_1(X_\tau)|$. Therefore, the $(|T_1(X_\tau)|-1)$-Capitulation of state $Z_1$ is the state $B_{2, 0}$. From Lemma~\ref{lemma:truncation},
\begin{equation}\locallabel{eq:z_1}
    r_{\lambda^*}(X_0', Z_1) + V(Z_1) \leq V(B_{2, 0}) + (|T_1(X_\tau)|-1)(1-\lambda^*).
\end{equation}
We are ready to upper bound $r_{\lambda^*}(X_0', X_\tau') + V(X_\tau')$:
\begin{align*}
    &r_{\lambda^*}(X_0', X_\tau') + V(X_\tau') = r_{\lambda^*}(X_0', X_\tau') + \alpha (r_{\lambda^*}(X_\tau', Z_1) + V(Z_1)) + (1-\alpha)(r_{\lambda^*}(X_\tau', Z_2) + V(Z_2))\\
    &\qquad= \alpha (r_{\lambda^*}(X_0', Z_1) + V(Z_1)) + (1-\alpha)(r_{\lambda^*}(X_0', Z_2) + V(Z_2)) \quad \text{From Observation~\ref{obs:path-independence}.}\\
    &\qquad\leq \alpha (V(B_{2, 0}) + (|T_1(X_\tau)|-1)(1-\lambda^*)) + (1-\alpha)(p-\lambda^*)|T_1(X_\tau)| \quad \text{From (\localref{eq:z_2}) and (\localref{eq:z_1}).}\\
    &\qquad= |T_1(X_\tau)|(\alpha(1-\lambda^*) + \alpha - (1-\alpha)\lambda^*) -\alpha(1-\lambda^*) + \alpha V(B_{2, 0})\quad \text{Substituting $p = \frac{\alpha}{1-\alpha}$.}\\
    &\qquad\leq |T_1(X_\tau)|(2\alpha - \lambda^*) + \alpha V(B_{2, 0})
\end{align*}
By assumption, $\sm$ is not optimal. Then $V(B_{2, 0})$
Assume for contradiction $\e{r_{\lambda^*}(X_0', X_{\tau'}') | E_3} > \e{r_{\lambda^*}(X_0, X_\tau) | E_3}$. Recall
$$\e{r_{\lambda^*}(X_0', X_{\tau'}') | E_1} \leq \e{r_{\lambda^*}(X_0, X_\tau) | E_1} \quad \text{(Claim~\localref{claim:3})}$$
and
$$\e{r_{\lambda^*}(X_0', X_{\tau'}') | E_2} \leq \e{r_{\lambda^*}(X_0, X_\tau) | E_2} \quad \text{(Claim~\localref{claim:4})}$$
Therefore, $V(B_{2, 0}) = \e{r_{\lambda^*}(X_0', X_{\tau'}')} \leq \e{r_{\lambda^*}(X_0', X_{\tau'}') | E_3}$. From the work above,
$$\e{r_{\lambda^*}(X_0', X_{\tau'}') | E_3} \leq \e{T_1(X_\tau) | E_3}(2\alpha -\lambda^*) + \alpha \e{r_{\lambda^*}(X_0', X_{\tau'}') | E_3}.$$

Thus,
$$V(B_{2, 0}) = \mathbb E[r(X_0', X_{\tau'}')] = \mathbb E[r(X_0', X_\tau') + V(X_\tau)] \leq \alpha V(B_{2, 0}) + (2\alpha - \lambda^*)\e{|T_1(X_\tau)|}.$$
Subtracting $\alpha V(B_{2, 0})$ from both sides, then dividing by $(1-\alpha)$, we get,
\begin{align*}
    V(B_{2, 0}) &\leq \e{|T_1(X_\tau)|}\frac{2\alpha - \lambda^*}{1-\alpha} = \e{|T_1(X_\tau)|} (1 - \lambda^*) + \e{|T_1(X_\tau)|}\frac{2\alpha - \lambda^* - 1 + \alpha + \lambda^* -\lambda^*\alpha}{1-\alpha}\\
    &\leq \e{|T_1(X_\tau)|} (1-\lambda^*) + \e{|T_1(X_\tau)|}\frac{3\alpha - \alpha\lambda^* - 1}{1-\alpha}\\
    &\leq \e{|T_1(X_\tau)|} (1-\lambda^*) + \e{|T_1(X_\tau)|}\frac{3\alpha - \alpha^2 - 1}{1-\alpha}\\
    &\leq \e{|T_1(X_\tau)|} (1-\lambda^*).
\end{align*}
From Lemma~\ref{lemma:selfish-mining-reward}, $\e{|T_1(X_\tau)|} = (2+\alpha/(1-2\alpha)$. This proves $V(B_{2, 0}) \leq (2+\alpha/(1-2\alpha))(1-\lambda^*)$.
\end{proof}
From Claim~\ref{claim:b_2_0}, $V(B_{2, 0}) \geq \big(2 + \frac{\alpha}{1-2\alpha}\big)(1-\lambda^*)$, and from Claim~\localref{claim:5}, $V(B_{2, 0}) \leq \big(2 + \frac{\alpha}{1-2\alpha}\big)(1-\lambda^*)$. This proves Proposition~\ref{prop:b_2_0}.
\end{proof}

\begin{claim}\label{claim:b_1_0}
If there is an optimal strategy that withhold block when Miner 1 wins block 1,
$$V(B_{1, 0}) \leq \frac{\alpha(1-\alpha)(2-3\alpha)}{1-2\alpha} + \alpha^2.$$
\end{claim}
\begin{proof}
Since Miner 1 withholds block 1, the game transitions to state $B_{2, 0}$ if Miner 1 wins block 2 or to state $V_{1, 1}$ if Miner 2 wins block 2. We get
\begin{align*}
V(B_{1, 0}) &= \alpha (r(B_{1, 0}, B_{2, 0}) + V(B_{2, 0})) + (1-\alpha) (r(B_{1, 0}, B_{1, 1}) + V(B_{1, 1}))\\
&= \alpha V(B_{2, 0}) + (1-\alpha) (V(B_{1, 1}) - \lambda^*)\\
&\leq \alpha \left(2 + \frac{\alpha}{1-2\alpha}\right)(1-\lambda^*) + (1-\alpha)\left(\frac{\alpha}{1-\alpha}-\lambda^*\right) \quad \text{From Claim~\ref{claim:b_1_1} and Proposition~\ref{prop:b_2_0}.}\\
&\leq \alpha \left(2 + \frac{\alpha}{1-2\alpha}\right)(1-\alpha) + (1-\alpha)\left(\frac{\alpha}{1-\alpha}-\alpha\right) \quad \text{Because $\lambda^* \geq \alpha$.}\\
&= \frac{\alpha(1-\alpha)(2-3\alpha)}{1-2\alpha} + \alpha^2.
\end{align*}
\end{proof}
\begin{lemma}\label{lemma:capitulate}
Suppose Miner 1 has an optimal strategy that capitulates to state $B_0$ once at state $B$. Then $V(B) = 0$.
\end{lemma}
\begin{proof}
Let $\pi$ be an optimal strategy where Miner 1 capitulates to state $B_0$ once at state $B$. Because Miner 1 capitulates to state $B_0$ at state $B$, starting from state $B_0$, Miner 1 can follow strategy $\pi$ as if they were at state $B$. Thus $0 = V(B_0) \geq V(B)$ (Lemma~\ref{lemma:bellman}). Similarly, starting from state $B$, Miner 1 can follow strategy $\pi$ as if they were at state $B_0$. Thus $V(B) \geq V(B_0) = 0$. Combining the inequalities proves $V(B) = 0$.
\end{proof}
\begin{proof}[Proof of Theorem~\ref{thm:nash-equilibrium}]\def\currentprefix{thm:nash-equilibrium}
The proof is by contrapositive: if there is an optimal strategy $\pi^*$ such that $\rev(\pi^*) > \alpha = \rev(\frontier)$, we will derive that $\alpha \geq 0.308$. From the Strong Recurrence Theorem~\ref{thm:strong-recurrence}, we can assume $\pi^*$ is checkpoint recurrent and positive recurrent.
\begin{claim}\label{claim:B_0_1}
If miner 2 wins block 1, $\pi^*$ capitulates at state $B_{0, 1}$ (and $V(B_{0, 1}) = 0$).
\end{claim}
\begin{proof}
Block 1 is a checkpoint since Miner 1 has no unpublished blocks. Because $\pi^*$ is checkpoint recurrent, Miner 1 capitulates at state $B_{0, 1}$. From Lemma~\ref{lemma:capitulate}, $V(B_{0, 1}) = 0$.
\end{proof}
\begin{claim}
If Miner 1 wins block 1, Miner 1 withhold block 1.
\end{claim}
\begin{proof}
Suppose for contradiction Miner 1 publishes block 1. Block 1 becomes a checkpoint and since $\pi^*$ is checkpoint recurrent, Miner 1 would capitulate at the next state. From Claim~\ref{claim:B_0_1}, we conclude Miner 1 always capitulates after the first round. This implies $\pi^* = \frontier$ and $\rev(\frontier) > \alpha$, a contradiction.
\end{proof}
We conclude that if Miner 1 creates block 1 the game goes to state $B_{1, 0}$ and if Miner 2 creates block 1, the game capitulates. Using the fact $\lambda^* = \rev(\pi^*) > \alpha$, we get
\begin{align*}
V(B_0) &= \alpha V(B_{1, 0}) + (1-\alpha)(V(B_{0, 1}) - \alpha)\\
&< \alpha V(B_{1, 0}) - \alpha(1-\alpha)\\
&\leq \frac{\alpha^2(1-\alpha)(2-3\alpha)}{1-2\alpha} + \alpha^3 - \alpha(1-\alpha).
\end{align*}
From Lemma~\ref{lemma:capitulate}, $V(B_0) = 0$. Solving the inequality, we get that $\alpha > 0.307979$.
\end{proof}

\end{document}
