# Supplementary material for: Proof-of-Stake Mining Games with Perfect Randomness
Source: arXiv:2107.04069 source file (2021-12-14)
Supplement: Supplementary file 7 [file trimming-appendix.tex]

\documentclass[class=article, crop=false]{standalone}

\input{../setup.tex}

\begin{document}
\subsection{Timeserving Reduction}
\subimport{./}{timeserving-proof.tex}

\subsection{Orderly Reduction}
\subimport{./}{orderly-proof.tex}

\subsection{Longest Chain Mining Reduction}
\subimport{./}{lcm-proof.tex}

\subsection{Trimmed Strategies}
\subimport{./}{trimmed-proof.tex}

\end{document}
